# Supplementary material for: An accurate solar axions ray-tracing response of BabyIAXO
Source: arXiv:2411.13915 source file (2024-11-29)
Supplement: Supplementary file 1 [file appendixY.tex]

The solution of the non-uniform magnetic field case is very similar to the development shown in the previous section. It is a popular topic in mathematics, named as "\emph{Linear Systems of Differential Equations with Variable Coefficients}"\footnote{https://www.math24.net/linear-systems-differential-equations-variable-coefficients/}. One requirement for the solution to be valid is that the matrix coefficients (i.e. the magnetic field in our case) must be continuous functions. 

\vspace{0.25cm}
We write the characteristic, or original, matrix as,

\begin{align*}
    \Upsilon(\tau)= -i \begin{pmatrix} r & B^\prime(\tau) \\ B^\prime(\tau) & s \end{pmatrix}
\end{align*}

\noindent where we must emphasize that the only variable parameter is the magnetic field, $B=B(\tau)$, being $\tau$ the parameterization of the position along the line-of-sight of the particle. For our particular case it has been checked the necessary condition that the coefficient matrix $\Upsilon$ commutes with its integral.

\vspace{0.25cm}
The general solution, or fundamental matrix, is given by the following expression,

\begin{align}\label{eq:PhiZ}
    \Phi(z) = \mbox{exp}\Big\{{\int_0^z \Upsilon(\tau)d\tau}\Big\}.
\end{align}

\noindent where we redefine the integral of the matrix as

\begin{align}\label{eq:IUpsilon}
    I_\Upsilon = \int_0^z \Upsilon(\tau)d\tau = -i \begin{pmatrix}
    rz & \int_0^z B^\prime d\tau \\
    \int_0^z B^\prime d\tau & sz
    \end{pmatrix}
     = -i \begin{pmatrix}
    rz & \tilde{B^\prime} \\
    \tilde{B^\prime} & sz
    \end{pmatrix}.
\end{align}

We have simplified the integral elements notation by introducing , $\tilde{B^\prime}=\int_0^z B^\prime d\tau$. We compute now the matrix exponential in expression~\ref{eq:PhiZ} by converting the matrix, shown in equation~\ref{eq:IUpsilon}, to its diagonal form. In this case, the coefficients depend on the variable $z$. The eigenvalues of this matrix, are obtained in a similar way as in the previous section leading to $\lambda_1\simeq-irz$ and $\lambda_2\simeq-isz$. The matrix of reduction to diagonal, $H$, is built using the corresponding eigenvectors,

\begin{align*}
H=
    \begin{pmatrix}
    \Theta z & \tilde{B^\prime} \\
    \tilde{B^\prime} & -\Theta z
    \end{pmatrix}.
\end{align*}

We need also the inverse matrix $H^{-1}$ that is calculated through the determinant $\Delta(H)$ and the transverse matrix,

\begin{align*}
    \Delta(H) = -\Theta^2 z^2 - \xcancel{\tilde{B^\prime}^2} = -\Theta^2z^2
\end{align*}

\noindent allowing to calculate the inverse as,

\begin{align*}
    H^{-1} = \frac{1}{\Delta(H)} H^T = \frac{1}{\Theta^2 z^2}     \begin{pmatrix}
    \Theta z & \tilde{B^\prime} \\
    \tilde{B^\prime} & -\Theta z
    \end{pmatrix}.
\end{align*}

We then obtain the Jordan form, rejecting terms in $\tilde{B^\prime}$ higher than 2,

\begin{align*}
    J = H^{-1} I_\Upsilon H = 
    \frac{-i}{\Theta^2 z^2}     \begin{pmatrix}
    \Theta z & \tilde{B^\prime} \\
    \tilde{B^\prime} & -\Theta z
    \end{pmatrix}
    \begin{pmatrix}
    rz & \tilde{B^\prime} \\
    \tilde{B^\prime} & sz
    \end{pmatrix}
    \begin{pmatrix}
    \Theta z & \tilde{B^\prime} \\
    \tilde{B^\prime} & -\Theta z
    \end{pmatrix}=\\
    = \frac{-i}{\Theta^2 z^2}
    \begin{pmatrix}
    \Theta r z^2 + \tilde{B^\prime}^2 & \tilde{B^\prime}rz \\
    \tilde{B^\prime}sz  & \tilde{B^\prime}^2 -\Theta s z^2
    \end{pmatrix}
    \begin{pmatrix}
    \Theta z & \tilde{B^\prime} \\
    \tilde{B^\prime} & -\Theta z
    \end{pmatrix} =\\
  =\frac{-i}{\Theta^2 z^2}\begin{pmatrix}
     \Theta^2 r z^3 + \xcancel{\tilde{B^\prime}^2 (\Theta  + r)z} & \xcancel{\tilde{B^\prime}^3}\\
     \xcancel{\tilde{B^\prime}^3} & \xcancel{\tilde{B^\prime}^2 (s-\Theta)z} + \Theta^2 s z^3 
    \end{pmatrix} \simeq -i
    \begin{pmatrix}
    rz & 0 \\
    0 & sz
    \end{pmatrix}
\end{align*}

Notice that the Jordan form was not exactly diagonal because the non-exact eigenvalues, but when we apply the transformation we obtain a matrix that is closer to the diagonal than it was the original matrix, $I_\Upsilon$, since the Jordan non-diagonal elements are of higher order, $\mathcal{O}(\tilde{B^\prime}^3)$.

The general solution will be given then by,

\begin{align*}
    \Phi(z)=H e^J H^{-1}=
    \frac{1}{\Theta^2 z^2} 
    \begin{pmatrix}
    \Theta z & \tilde{B^\prime} \\
    \tilde{B^\prime} & -\Theta z
    \end{pmatrix}
        \begin{pmatrix}
    e^{-irz} & 0 \\
    0 & e^{-isz}
    \end{pmatrix}
        \begin{pmatrix}
    \Theta z & \tilde{B^\prime} \\
    \tilde{B^\prime} & -\Theta z
    \end{pmatrix}=\\
    = \begin{pmatrix}
    1 & \tilde{B_\Theta^\prime} \\
    \tilde{B_\Theta^\prime} & -1
    \end{pmatrix}
        \begin{pmatrix}
    e^{-irz} & \tilde{B_\Theta^\prime}e^{-irz} \\
    \tilde{B_\Theta^\prime}e^{-isz} & -e^{-isz}
    \end{pmatrix}= 
    \begin{pmatrix}
    e^{-irz}+\tilde{B_\Theta^\prime}^2 e^{-isz} & \tilde{B_\Theta^\prime}( e^{-irz}-e^{-isz} ) \\
    \tilde{B_\Theta^\prime}( e^{-irz}-e^{-isz} ) & \tilde{B_\Theta^\prime}^2 e^{-irz}+e^{-isz}
    \end{pmatrix}
\end{align*}

\noindent where we have introduced the additional notation $\tilde{B_\Theta^\prime}=\tilde{B^\prime}/\Theta z$. The set of  solutions, $\Phi(z)$, after canceling terms $\mathcal{O}(\tilde{B_\Theta^\prime}^2)$, results in,

\begin{align*}
    \Phi(z)=\begin{pmatrix}
    e^{-irz} & \tilde{B_\Theta^\prime}( e^{-irz}+e^{-isz} ) \\
    \tilde{B_\Theta^\prime}( e^{-irz}-e^{-isz} ) & e^{-isz}
    \end{pmatrix}
\end{align*}.

We now build a general solution by introducing a linear combination of the solutions obtained at $\Phi(z)$, 

\begin{align*}
    A(z) = k_1 e^{-irz} + k_2 \tilde{B_\Theta^\prime}( e^{-irz}-e^{-isz} )
\end{align*}
\begin{align*}
   a(z) = k_1 \tilde{B_\Theta^\prime}( e^{-irz}-e^{-isz} )  + k_2 e^{-isz}
\end{align*}

\noindent and we impose the boundary conditions at the entrance of our helioscope, $A(z=0)=0$, which results in $k_1=0$, and $a(z=0)=1$, which results in $k_2=e^{isz}$. The solution for the EM-component reads finally,

\begin{align*}
    A(z) = \tilde{B_\Theta^\prime}( e^{-i\Theta z}-1 )
\end{align*}

\noindent which except for a phase it takes the same form as equation~\ref{eq:AzConstSol}, that will lead us to a solution very similar to the obtained with constant coefficients,

\begin{align}\label{eq:nonHomSolution}
    P_{a\gamma} = \frac{\left<B^\prime\right>^2}{q^2+\Gamma^2/4}\cdot \bigg\{ 1 + \mbox{exp}(-\Gamma L) -2\mbox{exp}(-\Gamma L/2)\mbox{cos}(qL)\bigg\}
\end{align}

\noindent where the field integral has been simply substituted by its average definition $\left<B^\prime\right>=\frac{1}{L}\int_0^L B^\prime d\tau$. Therefore, equation~\ref{eq:nonHomSolution} tells us that we can calculate the axion-photon conversion probability in the same way as we calculated the probability in the constant magnetic field case, we just need now to compute the average magnetic field integrated to the trajectory of the particle traversing the non-homogeneous magnetic field.

%%%%%%%%%%%%%%%%%%%%%%%%%%%%%%%%%%%%%%%%%%%%%%%%%%%%
%%%%%% Notes Maurizio   %%%%%%
%%%%%%%%%%%%%%%%%%%%%%%%%%%%%%%%%%%%%%%%%%%%%%%%%%%%

\section{Notes Maurizio on $a-\gamma$ oscillations}
\textbf{These are still preliminary notes.}

We want to solve the equation 
\begin{align}
\label{eq:ALP-gamma_oscillation}
\partial_z \psi =-iM(z)\psi
\end{align}
where
\begin{equation}
	M= \left(
		\begin{array}{cc}
		r & \Delta_{a\gamma} \\       
		\Delta_{a\gamma} & s\\
		\end{array}
	\right) = \frac12(r+s)\sigma_0+ \Delta_{a\gamma} \sigma_1 + \frac12(r-s)\sigma_3 \,.
\end{equation}
In the last step, we expanded in Pauli matrices plus identity ($\sigma_0$).
I find this a convenient way to represent $2\times 2$ hermitian matrices.

Often, the solution is expressed in terms of the transfer function $T(z)$, defined such that 
\begin{equation}
\psi(z)=T(z)\psi(0) \,.
\end{equation}

\subsection{Preliminary 1: A theorem about the solution of Eq.\eqref{eq:ALP-gamma_oscillation} }

Consider the linear homogeneous system of differential equations:
$$\dot \psi(t)=A(t) \psi(t)\,,$$
where $\psi$ is a vector, $\dot \psi$ its derivative with respect to $t$, and $A$ is a matrix. Let's define also the matrix
$$\phi(t)=\int_0^t A(\tau)d\tau\,,\qquad \Rightarrow \qquad \dot \phi(t)=A(t)\,.
$$
\textbf{Theorem}: 
$${\rm If}~~ [\dot \phi,\phi]=0 ~~ {\rm then}~~~ \psi(t)=e^{\phi(t)}\psi(0)\,.$$
To prove it, we expand the final result in Taylor series and differentiate it:
$$\dot\psi=\left[\sum_{n=1}^\infty \frac{1}{n!} \left(\frac{d}{dt}\phi^n \right)\right]\psi(0)\,.$$
If and only if $[\dot \phi,\phi]=0$ then $\frac{d}{dt}\phi^n=n \dot \phi\phi^{n-1}$. In this case, 
$$\dot\psi(t)=\dot \phi \left[\sum_{n=1}^\infty \frac{\phi^{n-1}}{(n-1)!} \right]\psi(0)
=A(t)\,e^{\phi(t)}\psi(0)=A(t)\psi(t)\,,$$ which proves the theorem. 
\subsection{Preliminary 2: Exponential of $2\times 2$ hermitian matrices}
\label{sec:preliminary_2}

Any hermitian matrix matrix can be expanded in Pauli matrices plus the identity:
$$M=x_0 \sigma_0+Q\,,\qquad  Q=\sum_{i=1}^3 x_i\sigma_i$$

Then, $e^{iMz}=e^{ix_0\sigma_0 z}e^{iQz}=(e^{ix_0 z}\sigma_0) e^{iQz}$. 
Using the properties of the Pauli matrices, it is easy to see that 
$$Q^{2n}=\xi^n \sigma_0\,, \qquad Q^{2n+1}=\xi^n Q\,,$$
with 
$$\xi=x_1^2+x_2^2+x_3^2\,.$$
Thus, 
\begin{align}
\label{eq:solution_MConstant}
	e^{iMz}=e^{i x_0 z}\left( \sum_{n=0}^\infty \frac{(iQz)^{2n}}{(2n)!}+
	\sum_{n=0}^\infty \frac{(iQz)^{2n+1}}{(2n+1)!} \right)=
	e^{i x_0 z}\left(\sigma_0\cos(z\sqrt{\xi})+
	\frac{iQ}{\sqrt{\xi}}\sin(z\sqrt{\xi})\right ) \,.
\end{align}

\subsection{Solution of Eq.\eqref{eq:ALP-gamma_oscillation} for constant $M$}

If $M$ is constant, then it definitely satisfies the theorem in the previous section and so the transfer function is simply
\begin{equation}
T(z)=e^{-i M z}=
e^{i x_0 z}\left(\cos(z\,\Delta_{\rm osc}/2)\sigma_0
	+i\frac{\sin(z\,\Delta_{\rm osc}/2)}{\Delta_{\rm osc}/2}Q 
	\right )
\,,
\end{equation}
where, following sec.~\ref{sec:preliminary_2}, $x_0=\frac12 (r+s)$, $Q=\Delta_{a\gamma}\sigma_1+ \frac12 (r-s)\sigma_3$, and $\xi=\Delta_{a\gamma}^2+\frac14(r-s)^2=\Delta_{\rm osc}$.\\

\textbf{Example: photon-axion oscillation probability}.
This probability is 
\begin{align}
	P_{a\gamma}=
\left|\left(e^{iMz}\right)_{12}\right|^2=
\Delta_{a\gamma}^2 \left(\frac{\sin (\Delta_{\rm osc}z/2)}{\Delta_{\rm osc}/2}\right)^2
\end{align}
where we used that $(\sigma_0)_{1,2}=0$ and $(Q)_{1,2}=x_1=\Delta_{a\gamma}$.

\subsection{General (non-homogeneous) case}

If the parameters in the matrix $M$ are not constant (for example, in the case of a non-uniform magnetic field), then we cannot use the simple exponential for the solution. 
In general, this case must be solved perturbatively. 

Let's start from Eq.~\eqref{eq:ALP-gamma_oscillation}.
Suppose that the off-diagonal term in $M$ is small (we should clarify the meaning of small). 
Then, we write $M(z)=H_0(z)+V(z)$
where $H_0=\frac12(r+s)\sigma_0+\frac12(r-s)\sigma_3$ is diagonal and $V=\Delta_{a\gamma}\sigma_1$ is small.
Explicitly,
\begin{align}
H_0 =	\left(
	\begin{array}{cc}
		\Delta_{\parallel}-i\frac{\Gamma}{2}  & 0 \\       
		0 & \Delta_a   \\
	\end{array}
	\right)\,,  \qquad
V =	\left(
\begin{array}{cc}
	0  & \Delta_{a\gamma} \\       
	\Delta_{a\gamma} & 0   \\
\end{array}
\right)\,,	
\end{align}
where the $\Delta$ are real and $ \Gamma $ is the damping coefficients (or inverse absorption length).
In principle, one should also add an imaginary contribution to the axion refractive index (that is, to $\Delta_a$).
However, the axion is extremely weakly coupled and we assume that it will not be reabsorbed.
Then, we can follow this strategy:
\begin{enumerate}
	\item Introduce  $$U(z)=e^{-i\int_0^z H_0(z^\prime)dz^\prime}$$
	Notice that $H_0$ is not hermitian and, consequently, $U$ is not a unitary matrix.
	\item Then, define $\psi_{\rm int}=U^{-1} \psi$, which will satisfy $i\partial_z \psi_{\rm int}=V_{\rm int}\psi_{\rm int}$, with $V_{\rm int}=U^{-1} V U$. 
	This can be solved perturbatively as $$i\partial_z \psi^{(n)}_{\rm int}=V_{\rm int}\psi^{(n-1)}_{\rm int}\,.$$
	\item At 0-th order, $V=0$ and $\psi^{(0)}(z)=U(z)\psi(0)~\Rightarrow ~ \psi^{(0)}_{\rm int}=\psi(0)$.
	\item At 1-st order, $i\partial_z \psi^{(1)}_{\rm int}=V_{\rm int}\psi^{(0)}_{\rm int}=U^{-1} V U \psi(0)$. 
	Thus, at this order of the perturbation in $V$, the solution of the equation is  
	\begin{align}
		\label{eq:evolution_weak_mixing}
		\psi(z)=\left[-iU\int_0^z U^{-1} V U \right]\psi(0)+U(z) \psi(0)\,,
	\end{align}
	which gives the transfer function (at the same order):
	\begin{align}
		\label{eq:transfer_function_weak_mixing}
		\boxed{T(z)=U(z)-iU(z)\int_0^z V_{\rm int}(z^{\prime})\,dz^{\prime}}
	\end{align}
\end{enumerate}

Let's proceed by defining $ U_\parallel = e^{iEz}e^{i\int_0^z \Delta_{\parallel} dz^\prime} $ and 
$ U_a=e^{iEz}e^{i\int_0^z \Delta_{a} dz^\prime}   $, so that
\begin{align}
U=	\left(
	\begin{array}{cc}
		U_\parallel
		e^{-\int_0^z \frac{\Gamma}{2} dz^\prime}  & 0 \\       
		0 &		U_a  \\
	\end{array}
	\right)\,.
\end{align}
From this definition, we find
\begin{align}
V_{\rm int}= U^{-1}VU=	-
\left(
\begin{array}{cc}
	0 & \Delta_{a\gamma} U_\parallel^\dagger U_a
	e^{\int_0^z \frac{\Gamma}{2} dz^\prime}  \\       
	\Delta_{a\gamma}^\dagger U_\parallel U_a
	e^{-\int_0^z \frac{\Gamma}{2} dz^\prime}  & 0 \\
\end{array}
\right)\,.
\end{align}
and
\begin{align}
	\label{eq:int_V_int_non_hermitian}
	\int_0^z	V_{\rm int}(z^{\prime}) \,dz^{\prime}= -
	\left(
	\begin{array}{cc}
		0  & G  \\
	  \tilde{G} & 0\\
	\end{array}
	\right)\,,
\end{align}
where 
\begin{align}
	& G=\int_0^z \Delta_{a\gamma}\, \left(
	\,e^{-i\int_0^{z^{\prime}} q(z^{\prime\prime}) dz^{\prime\prime}} 
	\, e^{\int_0^{z^{\prime}}  \frac{\Gamma(z^{\prime\prime})}{2} dz^{\prime\prime}} \right) \,dz^\prime \,,\\
	& \tilde G=\int_0^z \Delta_{a\gamma}\, \left(
	\,e^{i\int_0^{z^{\prime}} q(z^{\prime\prime}) dz^{\prime\prime}} 
	\, e^{-\int_0^{z^{\prime}}  \frac{\Gamma(z^{\prime\prime})}{2} dz^{\prime\prime}} \right) \,dz^\prime \,,\\
	& q=\Delta_\parallel -\Delta_a=\frac{m_a^2 - m_\gamma^2}{2\omega}\,.
\end{align}
Notice that $q$ is the momentum transferred, in the relativistic approximation $m_a\ll \omega$.

%\begin{align}
%& G=\int_0^z \Delta_{a\gamma}\, \left(
%	\,e^{-i\int_0^{z^{\prime}} \delta(z^{\prime\prime}) dz^{\prime\prime}} 
%	\, e^{\int_0^{z^{\prime}}  \frac{\Gamma(z^{\prime\prime})}{2} dz^{\prime\prime}} \right) \,dz^\prime \,,\\
%& \tilde G=\int_0^z \Delta_{a\gamma}\, \left(
%\,e^{i\int_0^{z^{\prime}} \delta(z^{\prime\prime}) dz^{\prime\prime}} 
%\, e^{-\int_0^z \frac{\Gamma}{2} dz^\prime} \right) \,dz^\prime \,,\\
%& \delta=\Delta_\parallel -\Delta_a=\frac{m_a^2 - m_\gamma^2}{2\omega}\,.
%\end{align}%also $R_{\pm}=(R\pm R^\dagger)/2$, $G_{\pm}=(G\pm G^\dagger)/2$.
%%
Finally,
\begin{align}
	T(z)= U+i
	\left(
	\begin{array}{cc}
		0  &  e^{-\int_0^z \frac{\Gamma}{2} dz^\prime}  U_{\parallel} G \\
	   U_{a} \tilde{G}  & 0\\
	\end{array}
	\right)\,,
\end{align}

\textbf{Example:} Let's calculate the axion-photon oscillation probability.
\begin{align}
&	P_{a\to A_\parallel}=
	|\langle A_\parallel(z)|a(0)\rangle|^2 =|T(z)_{1,2}|^2= \nonumber \\
&|U_\parallel|^2|G|^2e^{-\int_0^z \Gamma(z^\prime) dz^\prime} =|G|^2e^{-\int_0^z \Gamma(z^\prime) dz^\prime} =  \nonumber \\
&	e^{-\int_0^z \Gamma(z^\prime) dz^\prime}  \left| \int_0^z \Delta_{a\gamma}\, \left(
\,e^{-i\int_0^{z^{\prime}} q(z^{\prime\prime}) dz^{\prime\prime}} 
\, e^{\int_0^{z^{\prime}}  \frac{\Gamma(z^{\prime\prime})}{2} dz^{\prime\prime}} \right) \,dz^\prime \right|^2
\end{align}
Notice that this time $P_{a \to \gamma}\neq P_{\gamma\to a}$

%%%%%%%%%%%%%%%%%%%%%%%%%%%%%%%%%%%%%%%%%%%%%%%%%%%%
%%%%%% Additional remarks   %%%%%%
%%%%%%%%%%%%%%%%%%%%%%%%%%%%%%%%%%%%%%%%%%%%%%%%%%%%

%\section{Additional remarks}

%It is important to emphasize that the previous equation~\ref{eq:nonHomSolution} will only be valid as soon as the magnetic field function is continuous. If we leave a, lets say magnetic volume, where the field drops suddenly to zero, the equation will only be valid in the domain of the magnetic volume, and in order to propagate the field to other well defined magnetic volumes traversed by the particle-field we need to apply boundary conditions, and solve the equations again.

%Now, in the case we are considering, the amplitude of the axion field $a(z=L)$ is of order $B^\prime$, and therefore, the initial conditions at the second magnetic volume will be of order $A(z)\sim 1-B^\prime$, and $a(z)\sim B^\prime$. Since $B^\prime\ll1$, it is acceptable to consider that the initial conditions at the second volume are the same as the initial conditions at the first volume, and equation~\ref{eq:nonHomSolution} will be a good approximation of the axion-photon conversion probability at the second volume.

%The probability of axion-photon conversion after $N$ independent volumes could be expressed then as,

%\begin{align*}
%    P_{a\gamma} = \sum^N P_{a\gamma}^n
%\end{align*}

%\noindent where $P_{a\gamma}^n$ is the axion-photon probability calculated independently at each volume by equation~\ref{eq:nonHomSolution}. This relation will be valid as soon as the total probability remains low, $P_{a\gamma}\ll1$.
