# Supplementary material for: An accurate solar axions ray-tracing response of BabyIAXO
Source: arXiv:2411.13915 source file (2024-11-29)
Supplement: Supplementary file 2 [file appendixZ.tex]

We will start these developments from equation (11) found at reference\,\cite{PhysRevD.39.2089}. This equation describes the evolution of the axion, $a$, and electromagnetic field, $A$, and their mixing through the non-diagonal elements,

\vspace{0.25cm}

\begin{equation}\label{eq:main}
\partial_z \begin{pmatrix} A \\ a \end{pmatrix} = -i\begin{pmatrix} \begin{matrix} \omega-m_\gamma^2/2\omega-i\Gamma/2 & B/2M \\ B/2M & \omega - m_a^2/2\omega \end{matrix}  \end{pmatrix} \begin{pmatrix} A \\ a \end{pmatrix}.
\end{equation}

% \begin{equation}\label{eq:main}
% M = \begin{pmatrix} \begin{matrix} \omega-m_\gamma^2/2\omega-i\Gamma/2 & \frac12 g_{a\gamma} B_T^2 \\ \frac12 g_{a\gamma} B_T^2 & \omega - m_a^2/2\omega \end{matrix}  \end{pmatrix} 
% \end{equation}

\vspace{0.25cm}
\noindent This relation is the linearized version of the Klein Gordon equation, and we must be aware that it is only valid when $\omega\gg m_a^2 /2\omega$ and $\omega\gg|m_\gamma^2/2\omega+i\Gamma/2|$. Thus, this approximation would be problematic when $\omega\sim m_a$ or $\omega\sim m_\gamma$, which is by far not the case for axion helioscopes.

\vspace{0.25cm}

In order to simplify the calculations shown in the coming sections we will consider the following definitions
\begin{align*}
    r = \omega - m_\gamma/2\omega - i\Gamma/2 \quad\quad s = \omega - m_a^2/2\omega \quad\quad B^\prime = B/2M
\end{align*}
\begin{align*}
    \Theta = r - s = \frac{m_a^2 - m_\gamma^2}{2\omega}  - i\Gamma/2 = q - i\Gamma/2
\end{align*}

%%%%%%%%%%%%%%%%%%%%%%%%%%%%%%%%%%%%%%%%%%%%%%%%%%%%
%%%%%% Solution with constant coefficients.   %%%%%%
%%%%%%%%%%%%%%%%%%%%%%%%%%%%%%%%%%%%%%%%%%%%%%%%%%%%
%\section{Solution with constant coefficients.}

This section shows the solution with constant coefficients. Meaning that in our solution we will consider $B,\omega,m_a, m_\gamma,\Gamma,M=$cte. The general solution for equation\,\ref{eq:main} is the solution of an homogeneous system with constant coefficients, given by,

\begin{equation}\label{eq:general_solution}
\begin{pmatrix} A(z) \\ a(z) \end{pmatrix} = k_1 \mbox{exp}(\lambda_1 z)\begin{pmatrix} \xi_{11} \\ \xi_{21} \end{pmatrix} + k_2 \mbox{exp}(\lambda_2 z)\begin{pmatrix} \xi_{12} \\ \xi_{22} \end{pmatrix}.
\end{equation}

\noindent where $\lambda_{1,2}$ are the eigenvalues, and $\begin{pmatrix} \xi_{11} \\ \xi_{21} \end{pmatrix}$, \begin{pmatrix} \xi_{12} \\ \xi_{22} \end{pmatrix} are the eigenvectors of the characteristic matrix. Which can be obtained as follows,

\begin{align}
    \left| -i \begin{pmatrix} r & B^\prime  \\ B^\prime & s \end{pmatrix} -\lamdda \lambda \mathbb{1} \right| = \left( -ir - \lambda  \right)\left( -is - \lambda  \right) + \xcancel{B^\prime^2} = 0
\end{align}

\noindent resulting in $\lambda_1 \simeq -ir$ and $\lambda_2 \simeq -is$, and substituting those into the characteristic matrix we obtain for each eigenvalue its corresponding eigenvector.

\begin{align*}
    \lambda_1 \Rightarrow -i\begin{pmatrix} 0 & B^\prime  \\ B^\prime & -\Theta \end{pmatrix} \begin{pmatrix} \xi_{11} \\ \xi_{21}\end{pmatrix} = 0 \longrightarrow B^\prime \xi_{11} - \Theta \xi_{21} = 0
\end{align*}

\begin{align*}
    \lambda_2 \Rightarrow -i\begin{pmatrix} \Theta & B^\prime  \\ B^\prime & 0 \end{pmatrix} \begin{pmatrix} \xi_{12} \\ \xi_{22}\end{pmatrix} = 0 \longrightarrow \Theta \xi_{12} + B^\prime \xi_{22} = 0
\end{align*}

\begin{align*}
     \begin{pmatrix} \xi_{11} \\ \xi_{21}\end{pmatrix} = \begin{pmatrix} \Theta \\ B^\prime \end{pmatrix} \quad \quad \begin{pmatrix} \xi_{12} \\ \xi_{22}\end{pmatrix} = \begin{pmatrix} B^\prime \\ -\Theta \end{pmatrix}
\end{align*}

Using those relations, and replacing them at the equation~\ref{eq:general_solution} we obtain then the general solution for the electromagnetic component, $A(z)$, and the axion component, $a(z)$,

\begin{align}\label{eq:A_sol_cte}
    A(z) = k_1 \Theta\cdot  \mbox{exp}(-irz) + k_2 B^\prime \cdot \mbox{exp}(-isz)
\end{align}
\begin{align}\label{eq:a_sol_cte}
    a(z) = k_1 B^\prime\cdot  \mbox{exp}(-irz) - k_2 \Theta \cdot \mbox{exp}(-isz)
\end{align}

We now need to determine the value of $k_1$ and $k_2$ by imposing the boundary conditions at the entrance of our helioscope, $A(z=0)=0$ and $a(z=0)=1$. From relation~\ref{eq:A_sol_cte} we get,

\begin{align*}
    0 = k_1\Theta + k_2 B^\prime \quad \longrightarrow \quad k_1 = - \frac{B^\prime}{\Theta}k_2
\end{align*}

\noindent and replacing this expression on relation~\ref{eq:a_sol_cte} we get both coefficients,

\begin{align*}
    1 = k_1 B^\prime - k_2 \Theta = -k_2 \left( \frac{B^\prime^2}{\Theta}+\Theta\right) \quad \longrightarrow \quad k_2 = - \frac{\Theta}{\Theta^2+\xcancel{B^\prime^2}} \quad \mbox{and} \quad k_1 = \frac{B^\prime}{\Theta^2+\xcancel{B^\prime^2}}.
\end{align*}

\noindent that finally leads to the general expression for the electromagnetic field, $A(z)$, which is the component we are interested to detect,

\begin{align}\label{eq:AzConstSol}
    A(z) = \frac{B^\prime}{\Theta}\cdot \left[  \mbox{exp}(-irz) -  \mbox{exp}(-isz) \right] = -\frac{B^\prime}{\Theta}\mbox{exp}(-isz)\left[ 1-\mbox{exp}(-i\Theta z) \right].
\end{align}
%\begin{align}
%    a(z) =  \frac{B^\prime^2}{\Theta^2}\cdot  \mbox{exp}(-irz) +  %\mbox{exp}(-isz)
%\end{align}

We are interested on the probability the wave is found at a photon state component after a traveled distance, $L$. Therefore, we are interested to calculate $P_{a\gamma}=|A(z=L)|^2$, which results into

\begin{align*}
    P_{a\gamma}=\frac{B^\prime^2}{\Theta^2} \bigg\{ \Big[1-\mbox{exp}(-\Gamma L/2)\cdot \mbox{cos}(-qL) \Big]^2+\mbox{exp}(-\Gamma L) \cdot \mbox{sin}^2(-qL)\bigg\}=\\
    = \frac{B^\prime^2}{q^2+\Gamma^2/4}\cdot \bigg\{ 1 + \mbox{exp}(-\Gamma L) -2\mbox{exp}(-\Gamma L/2)\mbox{cos}(qL)\bigg\}
\end{align*}

\noindent which is the same relation as the one found at equation (16) in reference~\cite{PhysRevD.39.2089}.
